# Supplementary material for: Frontier models need only one text to unmask its human or AI author
Source: arXiv:2611.26216 source file (2026-11-28)
Supplement: Supplementary file 1 [file explanation_markers.tex]

\newcommand{\minjoonagent}[1]{{\color{orange!85!black}\{\textit{#1}\}$_{\text{minjoon-agent}}$}}
\newtcolorbox{minjoonagentblock}[1][]{enhanced, colback=orange!3, colframe=orange!85!black,
  boxrule=0.6pt, arc=1.5pt, left=3pt, right=3pt, top=2pt, bottom=3pt,
  title={\sffamily\scriptsize minjoon-agent}, toptitle=0pt, bottomtitle=0pt, #1}
\DeclareRobustCommand{\minjoonagentinline}[1]{{\color{orange!85!black}{\sffamily\footnotesize[minjoon-agent]}\ #1}}
